# Supplementary material for: An Improved Variational Approximate Posterior for the Deep Wishart Process
Source: arXiv:2305.14454 source file (2023-05-23)
Supplement: Supplementary file 1 [file uai2023-supplement.tex]

\documentclass[accepted]{uai2023}
\usepackage[british]{babel}

% for cross referencing the main text
% PLEASE ONLY USE xr IN THE SUPPLEMENTARY MATERIAL. 
% In the main paper, hard code any cross-reference to the supplementary material. 
\usepackage{xr} 

% making xr work on overleaf
\makeatletter
\newcommand*{\addFileDependency}[1]{% argument=file name and extension
\typeout{(#1)}% latexmk will find this if $recorder=0
\@addtofilelist{#1}
\IfFileExists{#1}{}{\typeout{No file #1.}}
}\makeatother

\newcommand*{\myexternaldocument}[2]{%
\externaldocument[#2]{#1}%
\addFileDependency{#1.tex}%
\addFileDependency{#1.aux}%
}

\usepackage{natbib}
    \bibliographystyle{plainnat}
    
\usepackage{mathtools} 
\usepackage{booktabs}
\usepackage[capitalize]{cleveref}
\usepackage{algorithm}
\usepackage{algorithmic}
\usepackage{xcolor}
\usepackage{tikz}
\usepackage{placeins}

%if overleaf, use this:
\myexternaldocument{uai2023-template}{}

%else:
%\externaldocument{uai2023-template}

\include{macros}

\author[1]{Sebastian Ober}
\author[2]{Ben Anson}
\author[2]{Edward Milsom}
\author[2]{Laurence Aitchison}
\affil[1]{%
    University of Cambridge
}
\affil[2]{%
    University of Bristol
}
  
\begin{document}
\input{appendix}

\FloatBarrier
\bibliography{uai2023-template}
% \bibliography
\end{document}
